# Supplementary material for: SeeThrough: Finding Chairs in Heavily Occluded Indoor Scene Images
Source: arXiv:1710.10473 source file (2017-12-04)
Supplement: Supplementary file 1 [file appendix.tex]

\appendix
\onecolumn
\section{Full results}
\label{app:results}
Results start on next page.
\begin{sidewaysfigure}[h!t]
    \includegraphics[width=\textwidth]{figures/qualitative_results/full/qual_results_0.pdf}
\end{sidewaysfigure}
\begin{sidewaysfigure}
    \includegraphics[width=\textwidth]{figures/qualitative_results/full/qual_results_1.pdf}
\end{sidewaysfigure}
\begin{sidewaysfigure}
    \includegraphics[width=\textwidth]{figures/qualitative_results/full/qual_results_2.pdf}
\end{sidewaysfigure}
\begin{sidewaysfigure}
    \includegraphics[width=\textwidth]{figures/qualitative_results/full/qual_results_3.pdf}
\end{sidewaysfigure}
\begin{sidewaysfigure}
    \includegraphics[width=\textwidth]{figures/qualitative_results/full/qual_results_4.pdf}
\end{sidewaysfigure}
\begin{sidewaysfigure}
    \includegraphics[width=\textwidth]{figures/qualitative_results/full/qual_results_5.pdf}
\end{sidewaysfigure}
\begin{sidewaysfigure}
    \includegraphics[width=\textwidth]{figures/qualitative_results/full/qual_results_6.pdf}
\end{sidewaysfigure}
\begin{sidewaysfigure}
    \includegraphics[width=\textwidth]{figures/qualitative_results/full/qual_results_7.pdf}
\end{sidewaysfigure}
\begin{sidewaysfigure}
    \includegraphics[width=\textwidth]{figures/qualitative_results/full/qual_results_8.pdf}
\end{sidewaysfigure}
\begin{sidewaysfigure}
    \includegraphics[width=\textwidth]{figures/qualitative_results/full/qual_results_9.pdf}
\end{sidewaysfigure}
\begin{sidewaysfigure}
    \includegraphics[width=\textwidth]{figures/qualitative_results/full/qual_results_10.pdf}
\end{sidewaysfigure}
\begin{sidewaysfigure}
    \includegraphics[width=\textwidth]{figures/qualitative_results/full/qual_results_11.pdf}
\end{sidewaysfigure}
\begin{sidewaysfigure}
    \includegraphics[width=\textwidth]{figures/qualitative_results/full/qual_results_12.pdf}
\end{sidewaysfigure}
\begin{sidewaysfigure}
    \includegraphics[width=\textwidth]{figures/qualitative_results/full/qual_results_13.pdf}
\end{sidewaysfigure}
\begin{sidewaysfigure}
    \includegraphics[width=\textwidth]{figures/qualitative_results/full/qual_results_14.pdf}
\end{sidewaysfigure}
\begin{sidewaysfigure}
    \includegraphics[width=\textwidth]{figures/qualitative_results/full/qual_results_15.pdf}
\end{sidewaysfigure}
\begin{sidewaysfigure}
    \includegraphics[width=\textwidth]{figures/qualitative_results/full/qual_results_16.pdf}
\end{sidewaysfigure}
\begin{sidewaysfigure}
    \includegraphics[width=\textwidth]{figures/qualitative_results/full/qual_results_17.pdf}
\end{sidewaysfigure}
\begin{sidewaysfigure}
    \includegraphics[width=\textwidth]{figures/qualitative_results/full/qual_results_18.pdf}
\end{sidewaysfigure}
\begin{sidewaysfigure}
    \includegraphics[width=\textwidth]{figures/qualitative_results/full/qual_results_19.pdf}
\end{sidewaysfigure}
\begin{sidewaysfigure}
    \includegraphics[width=\textwidth]{figures/qualitative_results/full/qual_results_20.pdf}
\end{sidewaysfigure}
\begin{sidewaysfigure}
    \includegraphics[width=\textwidth]{figures/qualitative_results/full/qual_results_21.pdf}
\end{sidewaysfigure}
\begin{sidewaysfigure}
    \includegraphics[width=\textwidth]{figures/qualitative_results/full/qual_results_22.pdf}
\end{sidewaysfigure}
