# Supplementary material for: SeeThrough: Finding Chairs in Heavily Occluded Indoor Scene Images
Source: arXiv:1710.10473 source file (2017-12-04)
Supplement: Supplementary file 2 [file supplementary.tex]

\section{Supplementary Materials}

\subsection{Amazon MTurk Annotation Interface and Keypoint Estimation} See Figure~\ref{fig:ch4:amt} for keypoint annotation (see Figure~\ref{fig:ch4:keypoint_types}) and corresponding network architecture is shown in Table~\ref{tab:ch4:network_architecture}. 

\begin{figure}[h!]
    \includegraphics[width=\linewidth]{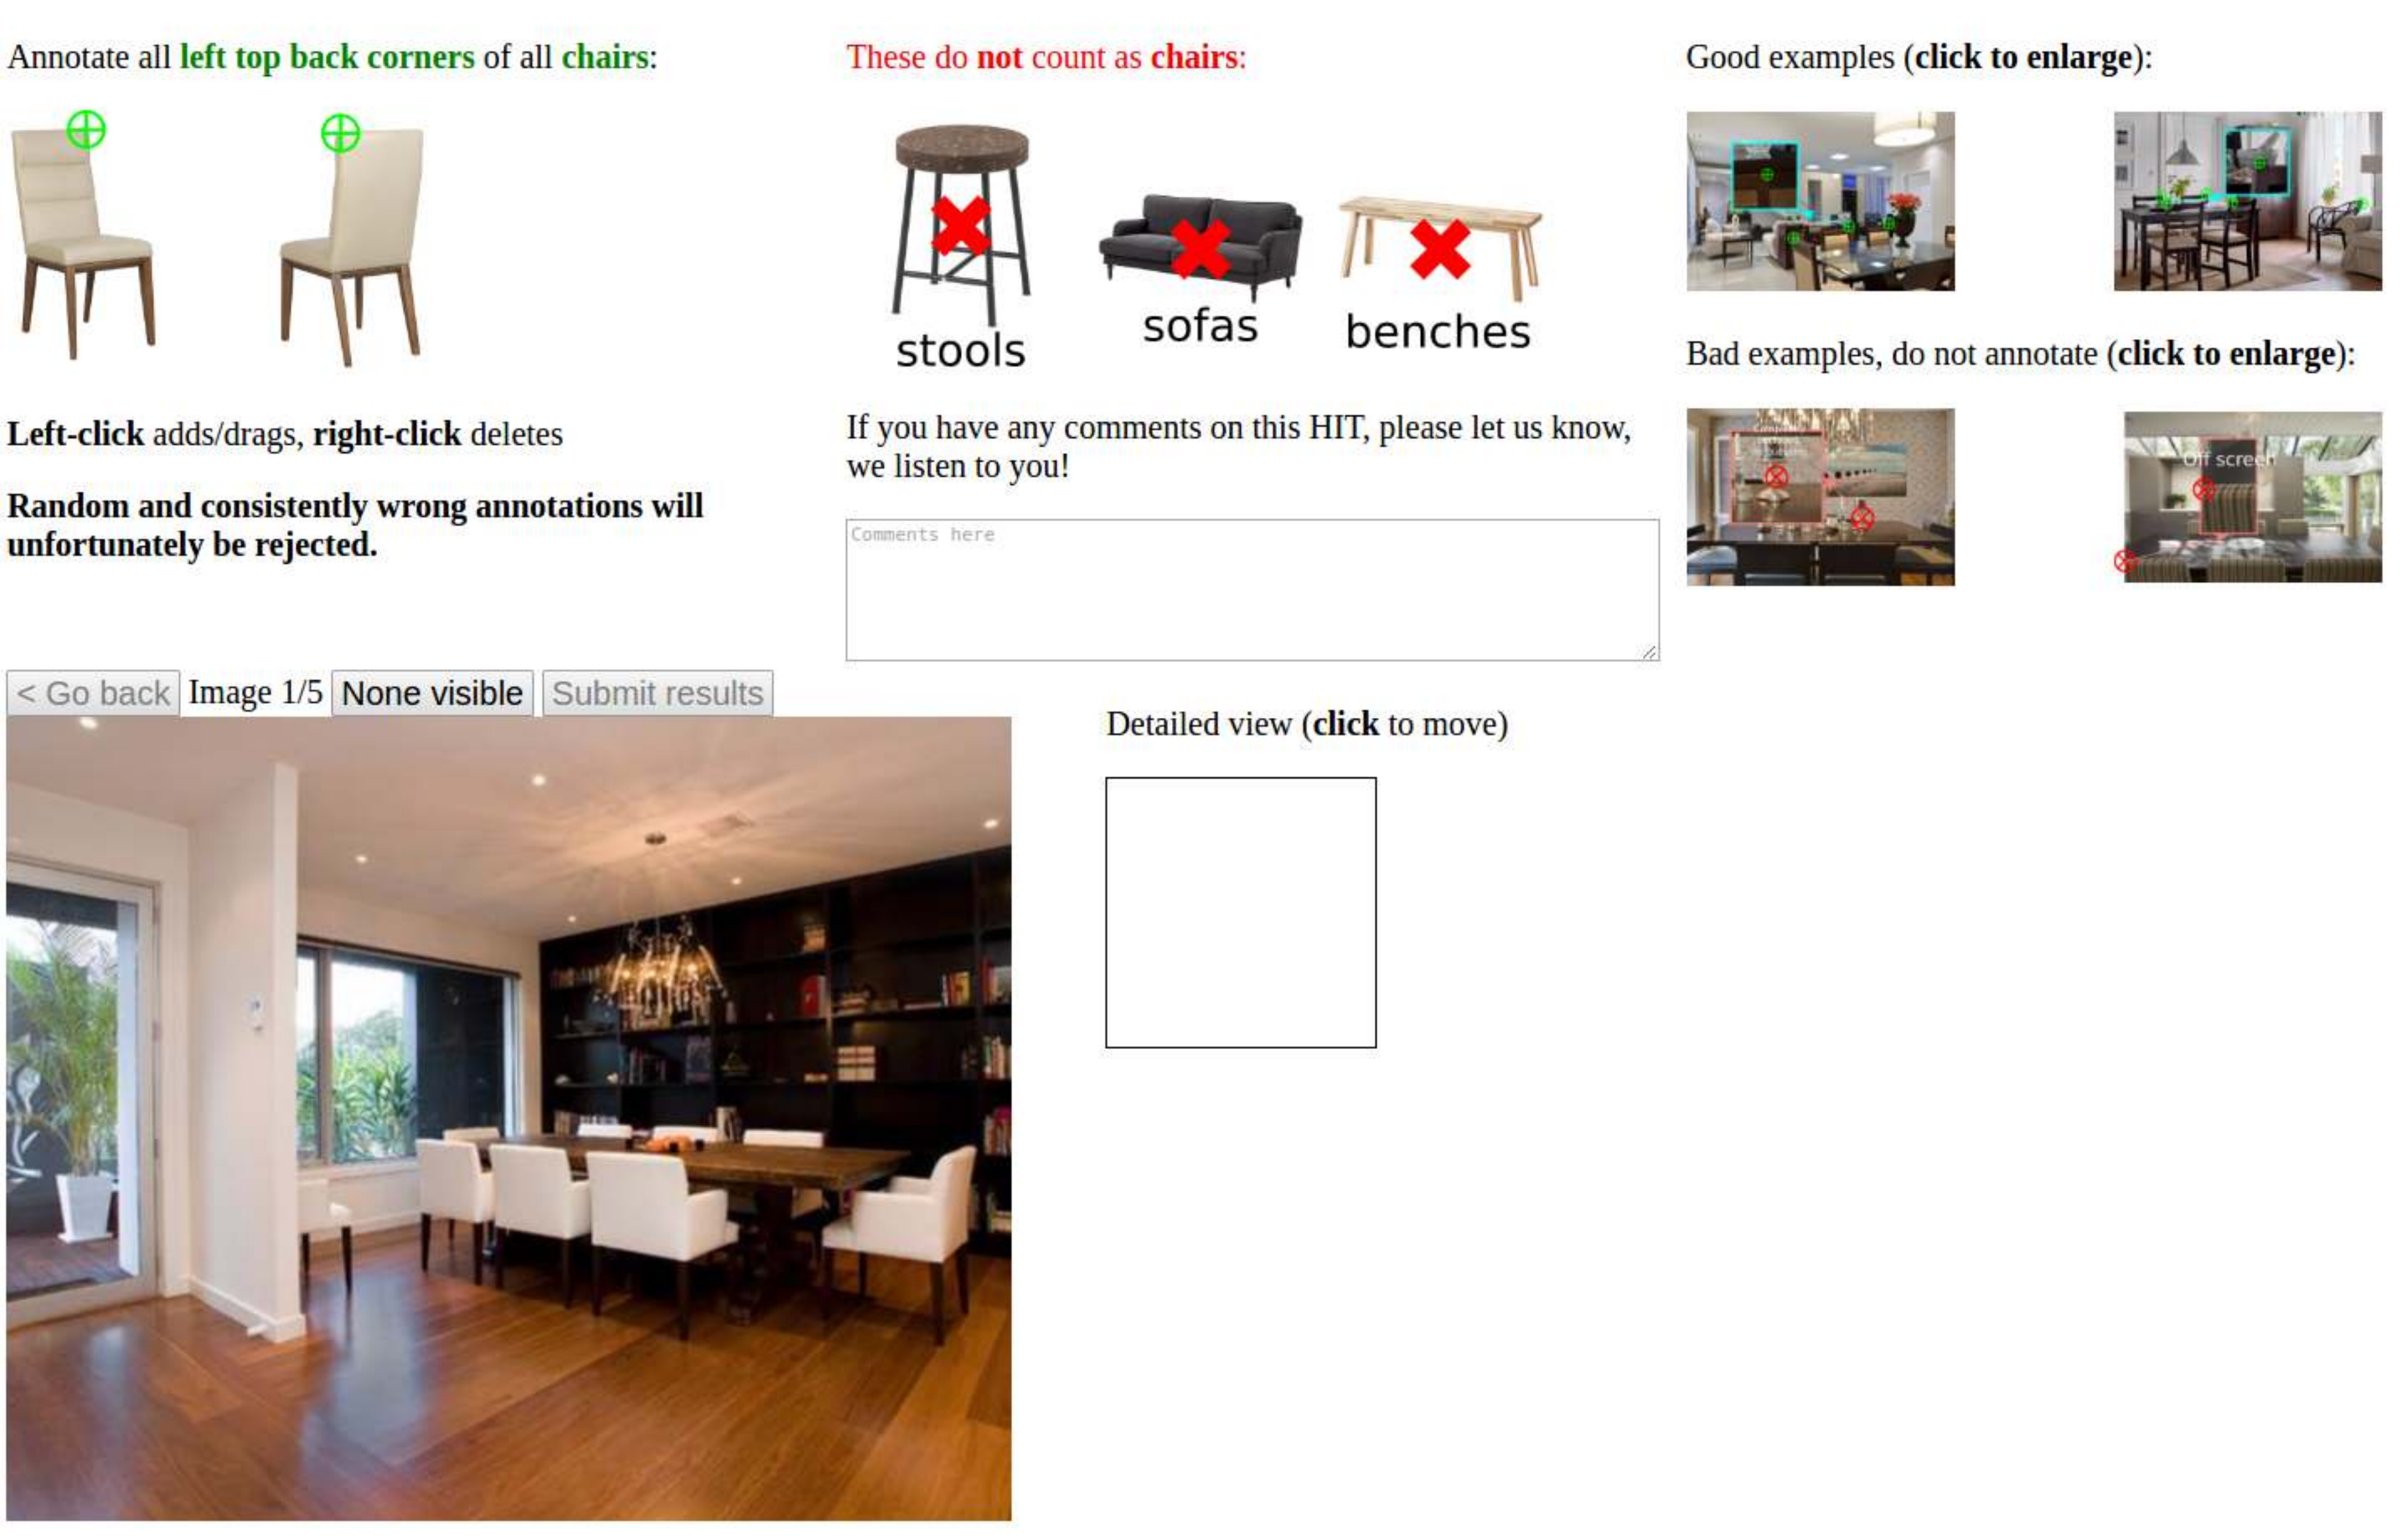}
    \caption{The Amazon MTurk interface we used to annotate 500 photographs with keypoints. Annotations were accepted if each image had consensus among 3 or more users.  }
    \label{fig:ch4:amt}
\end{figure}

\begin{table}[h!tb]
    \centering
    
    \caption{Network architecture used for keypoint estimation.}
    \label{tab:ch4:network_architecture}
    \resizebox{\linewidth}{!}{
        \bgroup
        
        \begin{tabular}{|c|c|c|}
            \hline
            layer name & output size & node type \\ \hline
            input      & $512 \times 512$ & \\ \hline
            conv\_1     & $256 \times 256$ & $7\times 7$, stride 2 \\ \hline
            max\_pool   & $128 \times 128$ & Max pooling, stride 2 \\ \hline
            block\_1 & $64 \times 64$ & Bottleneck units with shortcuts, $\begin{bmatrix} 1 \times 1, 64 \\ 3 \times 3, 64 \\ 1 \times 1, 256 \end{bmatrix} \times 3$, last $3\times 3$ stride 2 \MatTableStrut \\ \hline
            block\_2 & $64 \times 64$ & Bottleneck units with shortcuts, $\begin{bmatrix} 1 \times 1, 128 \\ 3 \times 3, 128 \\ 1 \times 1, 512 \end{bmatrix} \times 4$, all stride 1 \MatTableStrut \\ \hline
            block\_3 & $64 \times 64$ & Bottleneck units with shortcuts, $\begin{bmatrix} 1 \times 1, 256 \\ 3 \times 3, 256 \\ 1 \times 1, 1024 \end{bmatrix} \times 6$, all stride 1 \MatTableStrut \\ \hline
            block\_4 & $64 \times 64$ & Bottleneck units with shortcuts, $\begin{bmatrix} 1 \times 1, 512 \\ 3 \times 3, 512 \\ 1 \times 1, 2048 \end{bmatrix} \times 3$, all stride 1 \MatTableStrut \\ \hline
        \end{tabular}
        \egroup
    }
\end{table}

\subsection{Error Measures} In the following, we describe the error measures used to compare \SeeThrough\ with the baseline alternatives.

\begin{description}\itemsep0pt
    \item[Average Max IoU:] This measure takes a source scene and a target
        scene, and records the accuracy with which the volumes of the objects
        in the source scene agree with the objects in the target scene.
        Specifically, for each object in the source scene, we record the IoU of
        the object with its MaxIoU correspondence.  This measure is averaged
        over all objects in the source scene to produce the final measure. 

        \[ \mathrm{\AvgMaxIou}(\bb{S}, T) = \frac{1}{|\bb{S}|} \sum_{o_S \in \bb{S}} J_3(o_S, J_3^*(o_S, \bb{T})) \]

        We measure in both directions, i.e. with the ground truth as source and
        result as target, as well as vice versa.  The former can be thought of
        as a form of ``recall'' and the latter as a form of ``precision''. This
        measure is angle-agnostic and captures the location similarity of objects in the source
        scene w.r.t. those in the target scene.
    
    \item[Average Max 2D IoU:] This measures the average maximum IoU of the
        bounding boxes of each projected object in the source scene with the
        bounding boxes of the projected objects in the target scene.
        \[ \mathrm{\AvgMaxDIoU}(\bb{S}, \bb{T}) = \frac{1}{|\bb{S}|} \sum_{o_S \in \bb{S}} J_2(o_S, J_2^*(o_S, \bb{T})) \]    
    \item[Percentage correct location:] This measure takes a source scene and a
        target scene, and records the percentage of objects in the source scene
        that have a $J_3^*$ correspondence over a certain threshold
        $\tau_{J}$. To define it, we first set
        \begin{multline*}
            \mathrm{CorrectLoc}(\bb{S}, \bb{T}) = \\ \{ o_S \in \bb{S} \mid J_3(o_S, J_3^*(o_S, \bb{T})) > \tau_{J} \}.
        \end{multline*}
        Then,
        \[ \mathrm{\PctCorrLoc}(\bb{S}, \bb{T}) = \frac{|\mathrm{CorrectLoc}(\bb{S}, \bb{T})|}{|S|}. \]
        We again measure in both directions, yielding recall (ground truth is source, result is target)
        and precision (vice versa) measures.
        
    \item[Percentage correct:] As the previous measure, but with the added constraint that the
        angle difference is under a threshold $\tau_{\theta}$. So,
        \begin{multline*}
            \mathrm{CorrectFull}(\bb{S}, \bb{T}) = \\ \{ o_S \in \mathrm{CorrectLoc}(\bb{S}, \bb{T}) \mid \angle(o_S, J_3^*(o_S, \bb{T})) < \tau_{\theta} \}. 
        \end{multline*}
        Then,
        \[ \mathrm{\PctCorrFull}(\bb{S}, \bb{T}) = \frac{|\mathrm{CorrectFull}(\bb{S}, \bb{T})|}{|\bb{S}|}. \]
        
    \item[Angle difference:] This measures the average angle difference for the objects that have
        correct location. This measure is symmetrical.
        \begin{multline*}
            \mathrm{\AngDiff}(\bb{S}, \bb{T}) = \\ \frac{\sum_{o_S \in \mathrm{CorrectLoc}(\bb{S}, \bb{T})} \angle(o_S, J_3^*(o_S, \bb{T}))}{|\mathrm{CorrectLoc}(\bb{S}, \bb{T})|}
        \end{multline*}
\end{description}

\begin{figure}[h!]
    \includegraphics[width=\linewidth]{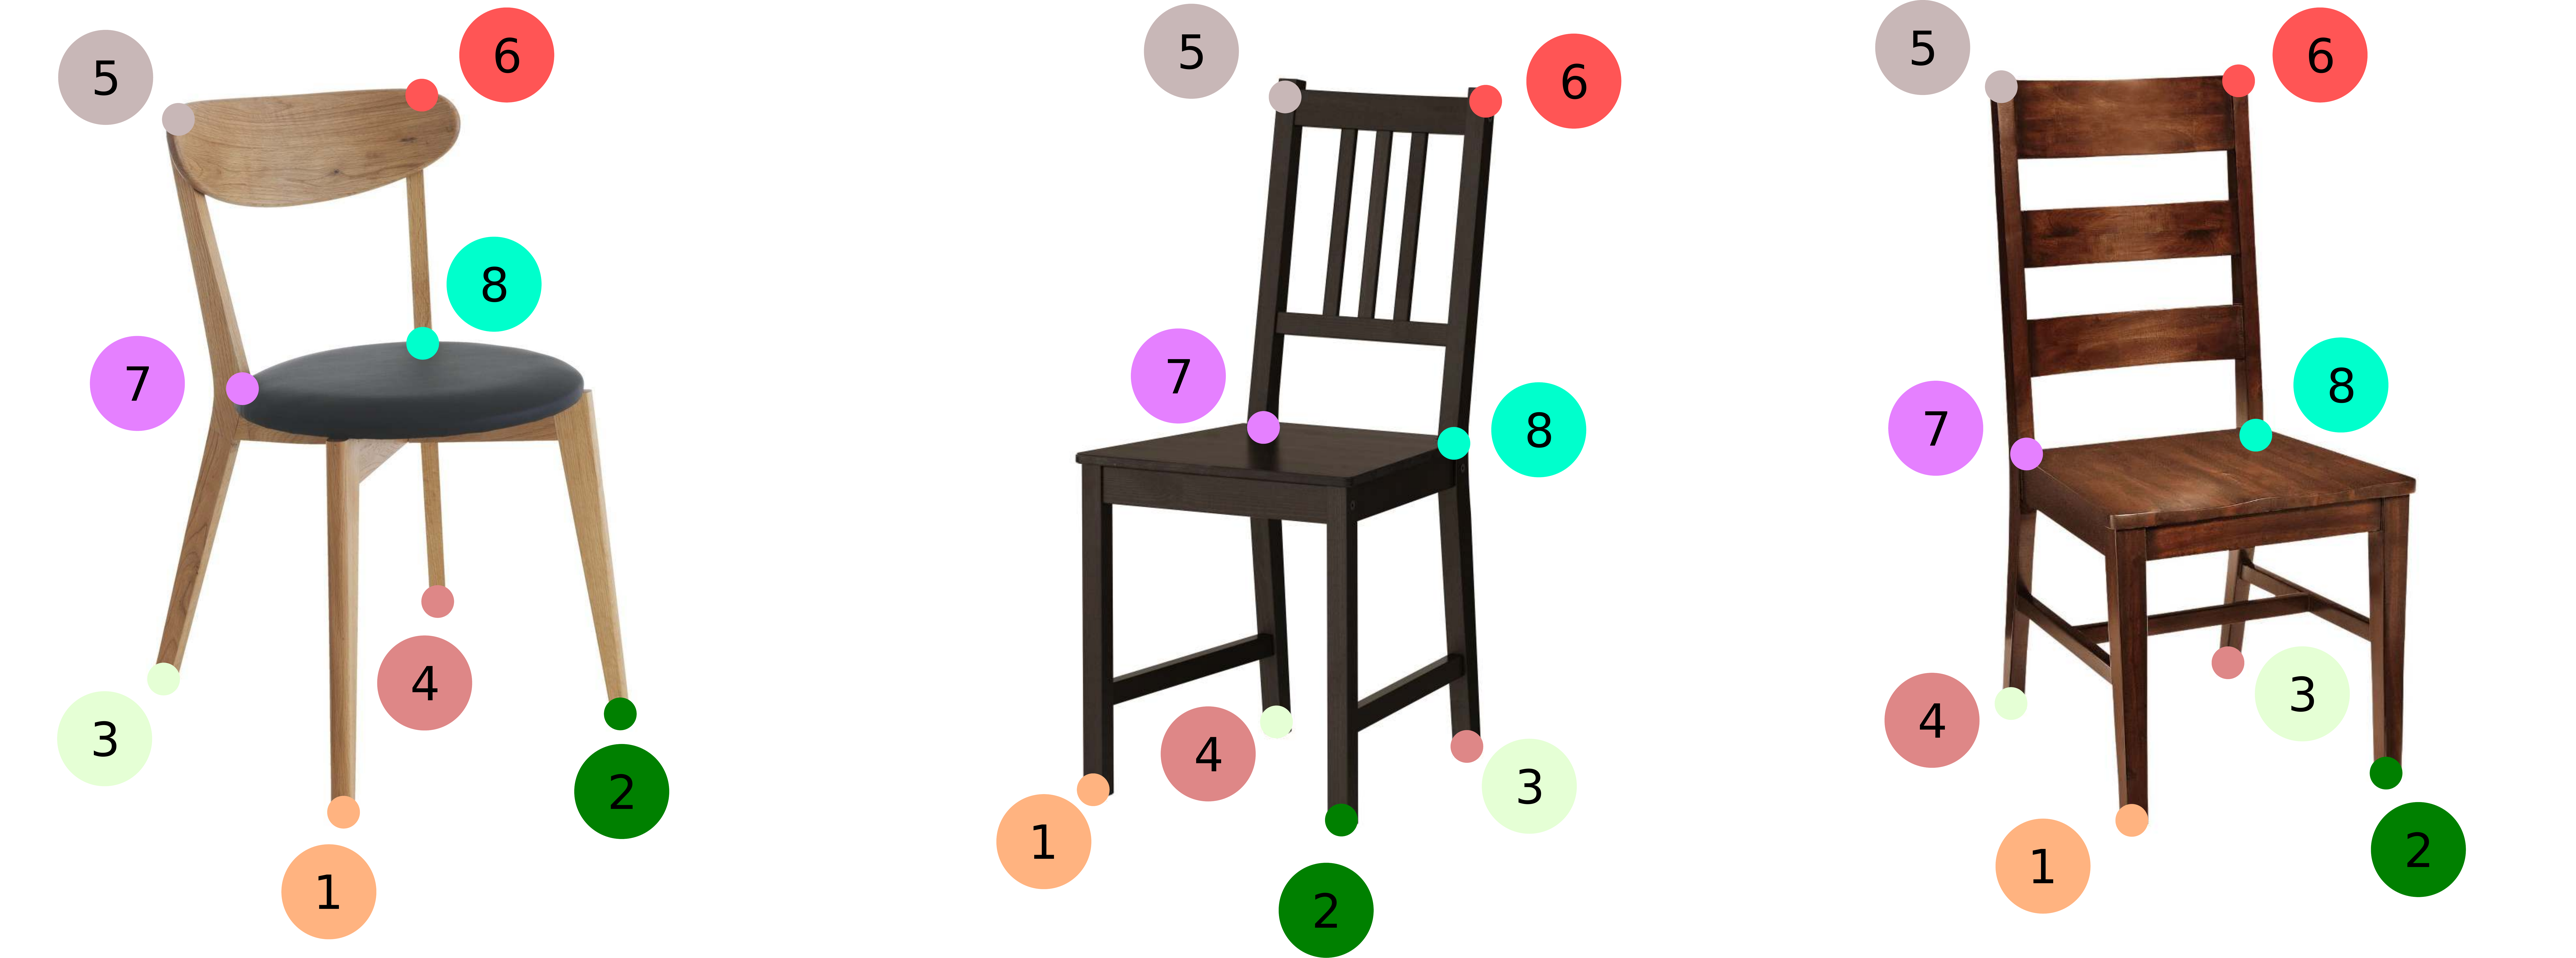}
    \caption[Keypoint types]{Selected keypoint types.}
    \label{fig:ch4:keypoint_types}
\end{figure}

\begin{figure}
    \includegraphics[width=\linewidth]{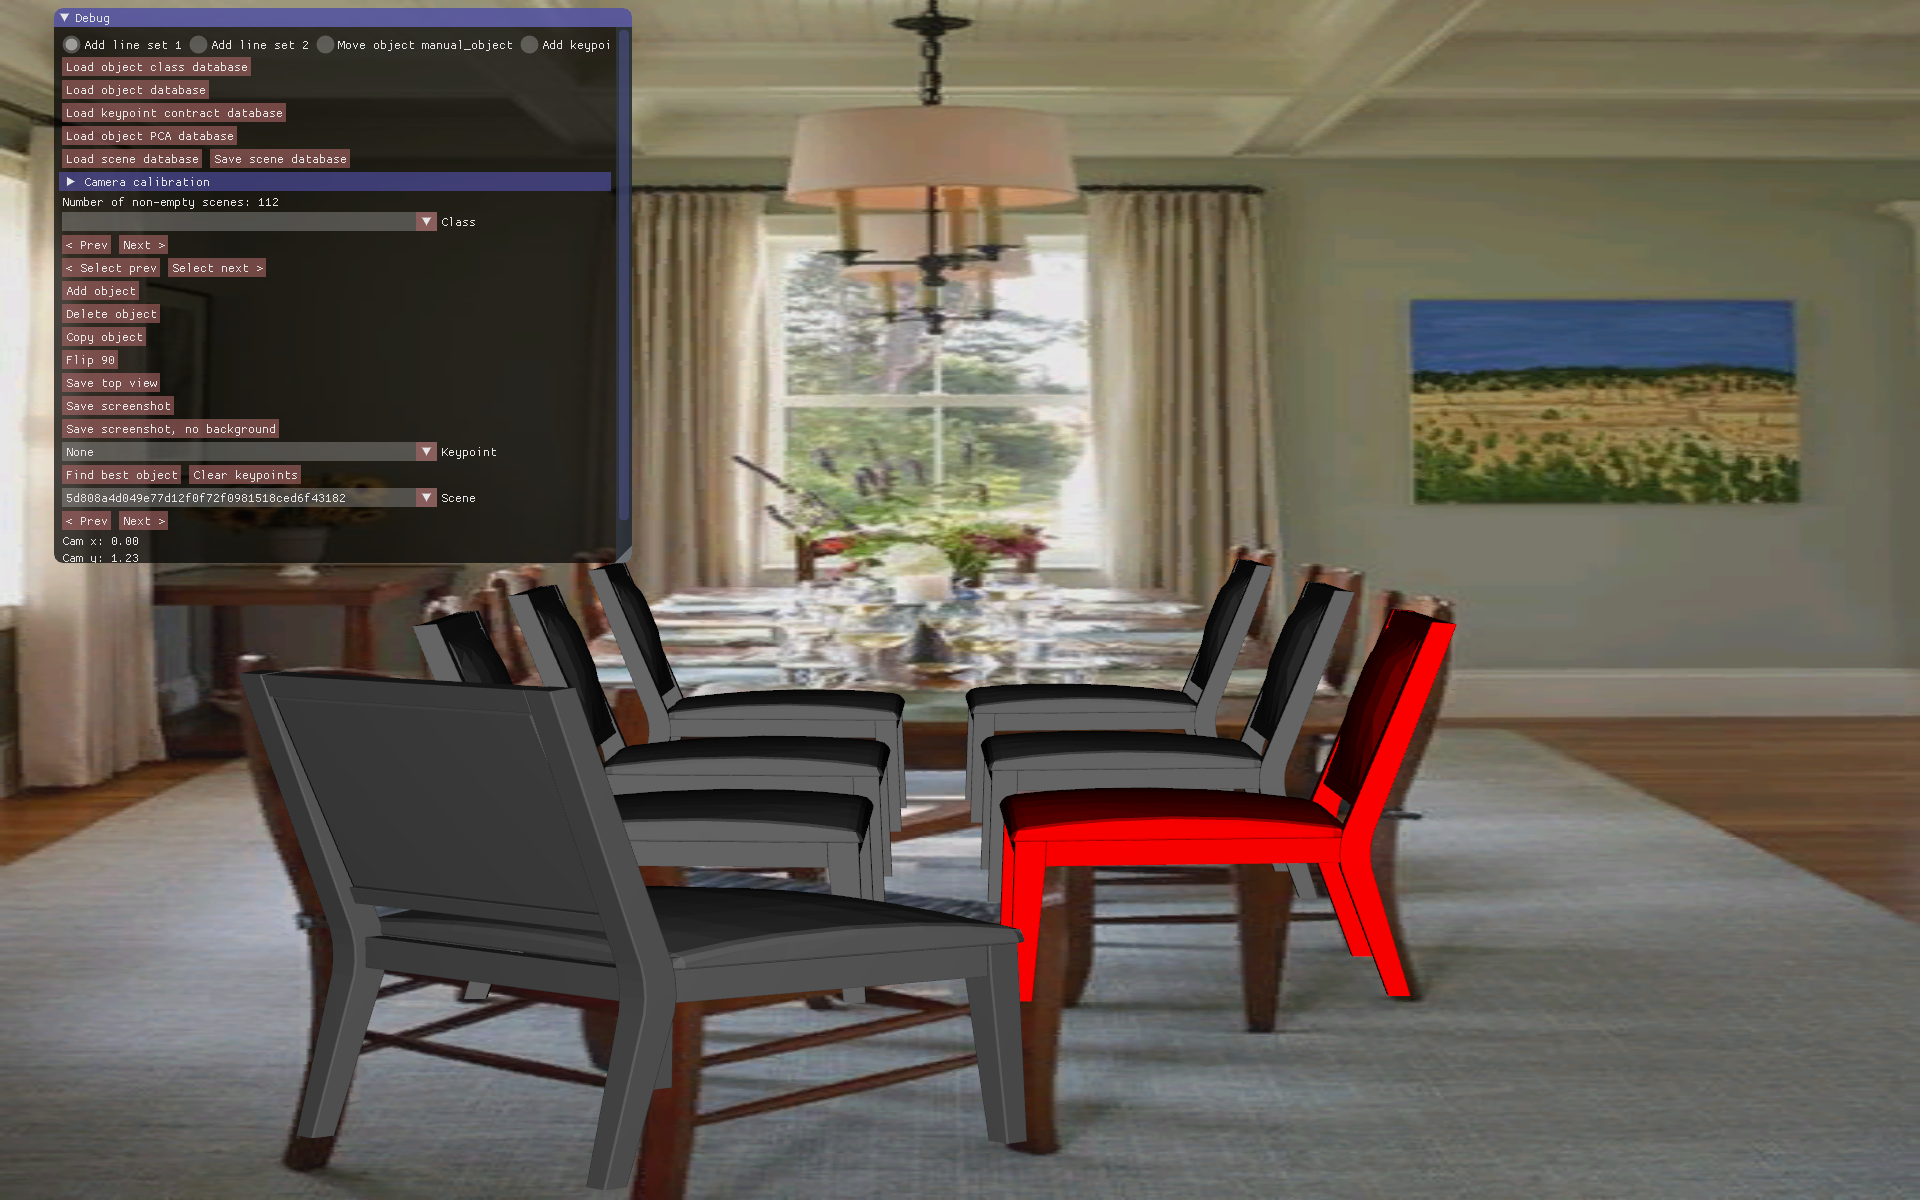}
    \caption[Annotation tool]{We created a ground truth annotation tool for quickly creating ground truth scene mockup examples.}
    \label{fig:ch4:gt_annotation}
\end{figure}

\subsection{Groundtruth Annotation Tool} We created a groundtruth annotation tool (see Figure~\ref{fig:ch4:gt_annotation}) for generating 3D mockup groundtruth to compare \SeeThrough\ with the baseline alternatives.

\begin{table}
    \centering
    \resizebox{\linewidth}{!}{
        \begin{tabular}{|c|c|c|}
            \hline
            Name     & Description                               & Value \\ \hline
            $\alpha$ & Sensitivity of keypoint maps              & 0.61  \\ \hline
            $\beta$  & Sensitivity to object co-occurrence model & 0.14  \\ \hline
            $\tau_m$ & Lower threshold of keypoint location map  & 0.25  \\ \hline
            $\tau_u$ & Maximum cost for selecting candidate      & 0.21  \\ \hline
        \end{tabular}
    }
    \caption[Hyper parameters]{Hyper parameters of optimization, found by HyperOpt~\cite{HyperOpt}.}
    \label{tab:ch4:hyperparameters}
\end{table}

\subsection{Qualitative Results} Please refer to supplementary files `topViewImages.pdf' and images in the folder `overlaidChairImages' (chairs shown in red and gray) for qualitative results. 
As shown in Figure~\ref{fig:ch4:baseline_example}, existing methods work well in regions where the objects are fully visible. But, since they rely on directly visible cues, the methods start failing under moderate to heavy occlusion (see Tables~\ref{tab:ch4:ablation} and \ref{tab:ch4:performance}). 

\begin{figure}[h!]
    \centering
    
    \import{figures/baseline_example/}{baseline_example.pdf_tex}
    \caption[Baseline output]{Example of raw output of the baseline methods.}
    \label{fig:ch4:baseline_example}
\end{figure}

\subsection{Hyperparameters}
Table~\ref{tab:ch4:hyperparameters} lists the parameters used in our experiments.

\begin{table*}[h!]
    \caption[Ablation study]{Ablation study showing the importance of using scene statistics and multiple iterations for best performance.}
    \resizebox{\linewidth}{!}{
        \begin{tabular}{|c|c|c|c|c|c|c|}
        \hline
                           & AvgMaxIOU (precision) & AvgMaxIOU (recall) & AvgMaxIOU (F1) & PercCorrectFull (precision) & PercCorrectFull (recall) & PercCorrectFull (F1) \\ \hline
        Full pipeline      & 0.386                 & 0.250              & \textbf{0.293} & 0.285                       & \textbf{0.161}           & \textbf{0.198} \\ \hline
        No scene stats     & 0.296                 & \textbf{0.265}     & 0.267          & 0.174                       & 0.151                    & 0.154 \\ \hline
        Single iteration   & \textbf{0.421}        & 0.190              & 0.251          & \textbf{0.346}              & 0.123                    & 0.175 \\ \hline
        \end{tabular}
        }
    \label{tab:ch4:ablation}
\end{table*}

\begin{table*}[h!]
\caption[Quantitative performance]{Quantitative performance of \SeeThrough\ versus the two baseline methods. We outperform the baselines significantly across all measures.}
    \resizebox{\linewidth}{!}{
          \begin{tabular}{|c|c|c|c|c|}
        \hline
                                                                      & \textsc{IoU3D} (precision)   & \textsc{IoU3D} (recall)   & \textsc{IoU3D} (F1)   & \\ \hline
        3D-INN~\cite{wu2016single} + FasterRCNN~\cite{Ren:2015:NIPS}  & 0.316                   & 0.150                & 0.198            & \\ \hline
        SeeingChairs~\cite{Aubry:2014:CVPR}                           & 0.195                   & 0.128                & 0.149            & \\ \hline
        Ours                                                          & \textbf{0.386}          & \textbf{0.250}       & \textbf{0.293}   & \\ \hline
                                                                      & \textsc{Loc} (precision) & \textsc{Loc} (recall) & \textsc{Loc} (F1) & \\ \hline
        3D-INN~\cite{wu2016single} + FasterRCNN~\cite{Ren:2015:NIPS}  & 0.263                   & 0.124                & 0.165            & \\ \hline
        SeeingChairs~\cite{Aubry:2014:CVPR}                           & 0.071                   & 0.043                & 0.052            & \\ \hline
        Ours                                                          & \textbf{0.298}          & \textbf{0.167}       & \textbf{0.207}   & \\ \hline
                                                                      & \textsc{LocAng} (precision) & \textsc{LocAng} (recall) & \textsc{LocAng} (F1) & \\ \hline
        3D-INN~\cite{wu2016single} + FasterRCNN~\cite{Ren:2015:NIPS}  & 0.04                        & 0.015                    & 0.021                & \\ \hline
        SeeingChairs~\cite{Aubry:2014:CVPR}                           & 0.013                       & 0.007                    & 0.009                & \\ \hline
        Ours                                                          & \textbf{0.285}              & \textbf{0.161}           & \textbf{0.198}       & \\ \hline
                                                                      & \textsc{IoU2D} (precision) & \textsc{IoU2D} (recall) & \textsc{IoU2D} (F1) & \textsc{AngDiff} (in degrees) \\ \hline
        3D-INN~\cite{wu2016single} + FasterRCNN~\cite{Ren:2015:NIPS}  & 0.526                   & 0.336                & 0.401            & 55.8                   \\ \hline
        SeeingChairs~\cite{Aubry:2014:CVPR}                           & 0.372                   & 0.325                & 0.341            & 11.4                   \\ \hline
        Ours                                                          & \textbf{0.628}          & \textbf{0.470}       & \textbf{0.525}   & \textbf{7.3}           \\ \hline

        \end{tabular}
    }
\label{tab:ch4:performance}
\end{table*}
